# Supplementary material for: Nonlinearly Stable Flux Reconstruction High-Order Methods in Split Form
Source: arXiv:2103.02647 source file (2021-03-03)
Supplement: Supplementary file 1 [file appendix.tex]

\section{Appendix}
